# Supplementary material for: PYROBOCOP : Python-based Robotic Control & Optimization Package for Manipulation and Collision Avoidance
Source: arXiv:2106.03220 source file (2021-06-06)
Supplement: Supplementary file 1 [file appendix.tex]

\subsection{Danskin's Theorem~\cite[Theorem 10.2.1]{FacchineiPangVol2}}\label{sec:danskinsthm}

Let $K \subseteq \R^m$ be 
a nonempty, closed set, $W \subseteq  \R^n$ be a 
nonempty, open set and $f : \R^n \times \R^m \rightarrow \R$ 
be continuous on $W \times K$. Consider the parametric 
optimization problem 
\[
    g(x) \equiv \inf\limits_{y \in K} f(x,y)
\]
for given values of the parameter $x \in W$.  The function $g(x) : W \rightarrow \R \cup \{-\infty\}$ is the optimal value function that is a function of only the parameters in the optimization problem. 
Danskin's theorem concerns the differentiability property of $g(x)$.  
We state the version of Danskin's theorem provided 
in~\cite[Theorem 10.2.1]{FacchineiPangVol2} with supremum replaced by 
infimum in order to be consistent with the formulation in this paper.

\begin{theorem}
Let $K \subseteq \R^m$ be a nonempty, closed set and let $W \subseteq  \R^n$ be a nonempty, open set. Assume that the function 
$f : W \times K \rightarrow \R$ is continuous on $W \times K$ 
and that $\nabla_x f(x, y)$ exists and is continuous on 
$W \times K$. Define the function 
$g : W \rightarrow \R \cup \{\infty\}$ by
\[
g(x) \equiv \inf\limits_{y \in K} f(x, y), x \in W
\]
and 
\[
M(x) \equiv \{y \in K \,|\, g(x) = f(x, y) \}.
\]
Let $x \in W$ be a given vector. Suppose that a neighborhood 
${\cal N}(x) \subseteq W$ of $x$ 
exists such that $M(x')$ is nonempty for all $x' \in {\cal N}(x)$ 
and the set $\cup_{x' \in {\cal N}(x)} M(x')$ is bounded. 
The following two statements (a) and (b) are valid.
\begin{enumerate}[(a)]
    \item The function $g$ is directionally differentiable at $x$ 
    and 
    \[
        g'(x;d) = \sup_{y \in M(x)} \nabla_x f(x, y)^T d.
    \]
    \item If $M(x)$ reduces to a singleton, say $M(x) = \{y(x)\}$, 
    then $g$ is G$\hat{\text{a}}$eaux differentiable at $x$ and
    \[
        \nabla g(x) = \nabla_x f(x, y(x)).
    \]
\end{enumerate}
\end{theorem}
